# Supplementary material for: Coherent optical-microwave interface for manipulation of low-field electronic clock transitions in $^{171}$Yb$^{3+}$:Y$_2$SiO$_5$
Source: arXiv:2209.04196 ancillary file (2022-09-09)
Supplement: Supplementary file 1 [file SI.pdf]

# SUPPLEMENTARY INFORMATION: Coherent optical-microwave interface for manipulation of low-field electronic clock transitions in $^{171}\text{Yb}^{3+}:\text{Y}_2\text{SiO}_5$

L. Nicolas,<sup>1,\*</sup> M. Businger,<sup>1</sup> T. Sanchez Mejia,<sup>1</sup> A. Tiranov,<sup>2</sup> T. Chanelière,<sup>3</sup>  
E. Lafitte-Houssat,<sup>4,5</sup> A. Ferrier,<sup>4,6</sup> P. Goldner,<sup>4</sup> and Mikael Afzelius<sup>1</sup>

<sup>1</sup>*Department of Applied Physics, University of Geneva, CH-1211 Geneva 4, Switzerland*

<sup>2</sup>*Center for Hybrid Quantum Networks (Hy-Q), The Niels Bohr Institute,  
University of Copenhagen, DK-2100 Copenhagen, Denmark*

<sup>3</sup>*Université Grenoble Alpes, CNRS, Grenoble INP, Institut Néel, 38000 Grenoble, France*

<sup>4</sup>*Chimie ParisTech, PSL University, CNRS, Institut de Recherche de Chimie Paris, 75005 Paris, France*

<sup>5</sup>*Thales Research and Technology, 91767 Palaiseau, France*

<sup>6</sup>*Faculté des Sciences et Ingénierie, Sorbonne Université, UFR 933, 75005 Paris, France*

## I. PERTURBATION CALCULATION OF THE EFFECT OF APPLYING A WEAK MAGNETIC FIELD

The  $^{171}\text{Yb}^{3+}$  ion has electronic  $S = \frac{1}{2}$ , and nuclear  $I = \frac{1}{2}$  spin and the effective spin Hamiltonian of both the ground and excited electronic levels of  $^{171}\text{Yb}^{3+}$  at zero magnetic field is

$$\mathcal{H}_0 = \mathbf{S} \cdot \mathbf{A} \cdot \mathbf{I}, \quad (\text{S.1})$$

where  $\mathbf{A}$  is the hyperfine coupling tensor. When a weak magnetic field  $\mathbf{B}$  is applied, one needs to add the effect of the Zeeman Hamiltonian  $\mathcal{H}_1 = \mathbf{B} \cdot \boldsymbol{\mu}$ , where  $\boldsymbol{\mu} = \mu_B \mathbf{g} \cdot \mathbf{S}$  is the magnetic moment. In the  $\text{Y}_2\text{SiO}_5$  crystal,  $^{171}\text{Yb}^{3+}$  ions replace  $\text{Y}^{3+}$  ions in sites of low ( $C_1$ ) point symmetry, which makes the hyperfine  $\mathbf{A}$  and Zeeman  $\mathbf{g}$  tensors highly anisotropic for both the ground and excited states. In general, for an  $\mathbf{A}$  tensor with non-zero eigenvalues  $A_x \neq A_y \neq A_z$ , the hyperfine coupling completely removes the degeneracy at zero magnetic field, giving rise to the four eigenstates,

$$\begin{aligned} |\psi^\pm\rangle &= \frac{1}{\sqrt{2}}(|\uparrow\downarrow\rangle \pm |\downarrow\uparrow\rangle), \\ |\phi^\pm\rangle &= \frac{1}{\sqrt{2}}(|\uparrow\uparrow\rangle \pm |\downarrow\downarrow\rangle), \end{aligned} \quad (\text{S.2})$$

where  $|\uparrow\rangle \equiv |S_z = \frac{1}{2}\rangle$ ,  $|\downarrow\rangle \equiv |S_z = -\frac{1}{2}\rangle$  are electronic spin components and  $|\uparrow\rangle \equiv |I_z = \frac{1}{2}\rangle$ ,  $|\downarrow\rangle \equiv |I_z = -\frac{1}{2}\rangle$ , the nuclear spin components. The eigenstates of  $\mathcal{H}_0$  are thus *Bell states* in the up and down spin states of the electronic and nuclear spin components. Their eigen energies are expressed as

$$\begin{aligned} E_{\phi^\pm} &= \frac{1}{4} [A_z \pm (A_x - A_y)], \\ E_{\psi^\pm} &= \frac{1}{4} [-A_z \pm (A_x + A_y)]. \end{aligned} \quad (\text{S.3})$$

Fig. S1 shows the energy level diagram and the corresponding eigenstates, taking  $\mathbf{A}$ -tensor diagonal elements  $A_x = -0.13$  GHz,  $A_y = 1.18$  GHz and  $A_z = 4.87$  GHz [1] (for site II). Note that the diagonal  $\mathbf{g}$  tensor are  $g_x = 0.13$ ,  $g_y = 1.5$  and  $g_z = 6.06$  [2].

### A. Definition of the $S_1$ gradient

Here, we will analytically derive an approximate formula to calculate the transition field-gradient  $S_1$ , when applying a weak magnetic bias field in an arbitrary direction, based on a first-order perturbation approach. In the analytical

---

\* Email to: [louis.nicolas@unige.ch](mailto:louis.nicolas@unige.ch)

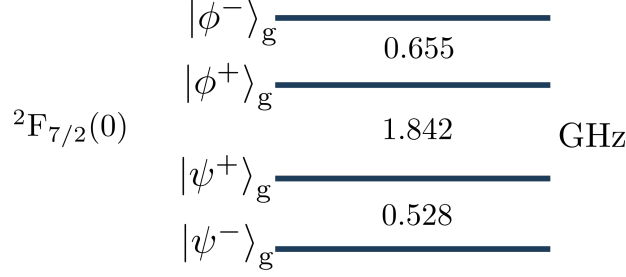

FIG. S1. Energy level diagram of the ground state of  $^{171}\text{Yb}^{3+}:\text{Y}_2\text{SiO}_5$

calculations, we will assume that the tensors  $\mathbf{A}$  and  $\mathbf{g}$  are aligned (i.e. diagonal in the same basis), which is a rather good approximation for the ground and excited levels of  $^{171}\text{Yb}^{3+}$  in  $\text{Y}_2\text{SiO}_5$  [1].

We assume a bias magnetic field is applied in an arbitrary direction  $\mathbf{B} = (B_x, B_y, B_z)$ . The goal is to calculate the linear sensitivity to a magnetic noise field, given that we have applied a bias field  $\mathbf{B}$ . Given a transition  $T$  between two energy levels, for instance  $T = E_{\psi^+} - E_{\psi^-}$ , the  $S_1$  gradient is calculated by taking the derivative of  $T$  as a function of the magnetic field in the  $x$ ,  $y$  and  $z$  directions [3], and from which we then calculate the norm of the corresponding gradient vector

$$S_1 = \sqrt{\left(\frac{dT}{dB_x}\right)^2 + \left(\frac{dT}{dB_y}\right)^2 + \left(\frac{dT}{dB_z}\right)^2}. \quad (\text{S.4})$$

Hence, we need to calculate the change in energy of a state as a function of a small perturbing field  $dB_k$ , for  $k = x, y, z$ , given the applied bias field  $\mathbf{B}$ .

### B. Two-step perturbation calculation

We take a two-step perturbative approach. We assume that an energy level has an unperturbed eigenstate  $|\chi\rangle$ , i.e. it is an eigenstate to  $\mathcal{H}_0$  listed in Eq. S.2. In the first step, we calculate the perturbed eigenstate  $|\tilde{\chi}\rangle$  due to the applied bias field  $\mathbf{B}$ . In the second step, we use the perturbed eigenstate to do a first-order perturbation of the eigenenergy  $E_\chi$  due to a smaller noise field  $dB_k$ .

In the first step, we consider a perturbing Hamiltonian  $\mathcal{H}_1$  due to the electronic Zeeman effect, where  $\mathcal{H}_1 = \mu_B \mathbf{B} \cdot \mathbf{g} \cdot \mathbf{S}$ . Note that, in principle, we should write a tensorial product  $\mathbf{S} \otimes 1$ , as  $\mathbf{S}$  only acts on the electronic spin and leaves the nuclear spin unaffected. However, we use a more compact notation throughout this note, where it is implicit that any  $S_k$  ( $k = x, y, z$ ) spin half operator acts only on the electronic spin. As stated above, we assume that  $\mathbf{A}$  and  $\mathbf{g}$  are aligned, and we work in the diagonal basis of both. Then, we can simply write out  $\mathcal{H}_1$  as

$$\mathcal{H}_1 = \mu_B B_x g_x S_x + \mu_B B_y g_y S_y + \mu_B B_z g_z S_z. \quad (\text{S.5})$$

The first-order perturbation of any eigenstate  $|\chi\rangle$  to  $\mathcal{H}_0$ , due to  $\mathcal{H}_1$ , is given by

$$|\tilde{\chi}\rangle \approx |\chi\rangle + \sum_{\alpha \neq \chi} \frac{\langle \alpha | \mathcal{H}_1 | \chi \rangle}{E_\chi - E_\alpha} |\alpha\rangle = |\chi\rangle + \sum_{\alpha \neq \chi} \kappa_\alpha \gamma_{\alpha\chi} |\alpha\rangle, \quad (\text{S.6})$$

where  $\kappa_\alpha = 1/(E_\chi - E_\alpha)$  and  $\gamma_{\alpha\chi} = \langle \alpha | \mathcal{H}_1 | \chi \rangle$ . Note that  $|\alpha\rangle$  in the sum is running over all the other Bell states in Eq. S.2, except  $|\chi\rangle$ .

In the second step of the perturbation calculation, we assume a smaller perturbing noise field in a given direction  $dB_k$  ( $k = x, y, z$ ). The associated perturbing Hamiltonian  $\mathcal{H}_2$  is then

$$\mathcal{H}_2 = \mu_B dB_k g_k S_k. \quad (\text{S.7})$$

We note here that the first-order energy shift of  $|\chi\rangle$  due to  $\mathcal{H}_2$  is zero, as  $\langle\chi|S_k|\chi\rangle = 0$ . This is the fundamental reason why we first need to perturb the eigenstate to first order due to the bias-field Hamiltonian  $\mathcal{H}_1$ , i.e. calculate  $|\tilde{\chi}\rangle$ , and then calculate the first-order energy shift due to  $\mathcal{H}_2$  with respect to  $|\tilde{\chi}\rangle$ ,

$$dE_\chi = \langle\tilde{\chi}|\mathcal{H}_2|\tilde{\chi}\rangle = \mu_B dB_k g_k \langle\tilde{\chi}|S_k|\tilde{\chi}\rangle, \quad (\text{S.8})$$

which gives the gradient along the  $k$  direction

$$\frac{dE_\chi}{dB_k} = \mu_B g_k \langle\tilde{\chi}|S_k|\tilde{\chi}\rangle. \quad (\text{S.9})$$

Hence, the calculation of  $S_1$  boils down to evaluate  $\langle\tilde{\chi}|S_k|\tilde{\chi}\rangle$  for  $k = x, y, z$ , which we will do to first-order in section ID. Note also that the first-order  $^{171}\text{Yb}^{3+}$  effective magnetic dipole moment vector can then be written as

$$\langle\boldsymbol{\mu}\rangle = \mu_B (g_x \langle\tilde{\chi}|S_x|\tilde{\chi}\rangle, g_y \langle\tilde{\chi}|S_y|\tilde{\chi}\rangle, g_z \langle\tilde{\chi}|S_z|\tilde{\chi}\rangle). \quad (\text{S.10})$$

### C. Effective magnetic dipole moment, dipole-dipole interaction and ESEEM

We briefly discuss the effective magnetic dipole moment due to the electronic spin component,  $\boldsymbol{\mu} = \mu_B \mathbf{g} \cdot \mathbf{S}$ , and the implications for dipole-dipole interactions.

Without the bias field, i.e. at the ZEFOZ point  $\mathbf{B} = 0$ , to first order all the vector components of the dipole moment  $\langle\boldsymbol{\mu}\rangle$  is zero with respect to the unperturbed eigenstates, as we have  $\langle\chi|S_k|\chi\rangle = 0$ . This implies that any dipole-dipole coupling with neighbouring  $\text{Y}^{3+}$  ions, i.e. superhyperfine interactions, vanish to first order. Specifically, in Ref. [4] it was shown that to first order the dipole-dipole coupling to neighboring  $\text{Y}^{3+}$  can be written as a function of the expectation value of the dipole moment operator. To account for the dipole-dipole interaction and the Zeeman effect of the yttrium ion, we need to add the following Hamiltonian to the ytterbium  $^{171}\text{Yb}^{3+}$  Hamiltonian:

$$\mathcal{H}_Y = \boldsymbol{\mu}_Y \cdot \left( \mathbf{B} - \frac{\mu_0}{4\pi} \left[ \frac{\langle\boldsymbol{\mu}\rangle}{r^3} - 3 \frac{(\langle\boldsymbol{\mu}\rangle \cdot \mathbf{r}) \cdot \mathbf{r}}{r^5} \right] \right) = \boldsymbol{\mu}_Y \cdot \mathbf{B}_Y, \quad (\text{S.11})$$

where  $\boldsymbol{\mu}_Y$  is the dipole moment of the  $\text{Y}^{3+}$  ion,  $\mathbf{r}$  the vector joining the  $^{171}\text{Yb}^{3+}$  ion to the  $\text{Y}^{3+}$  ion ( $r$  is its norm), and  $\mu_0$  the vacuum permeability. The second term in the equation for  $\mathbf{B}_Y$  above can be interpreted as the magnetic field produced by the ytterbium ion on the yttrium ion, which changes the norm and orientation of the effective local magnetic field on the yttrium ion. The effect of this term is to allow so-called nuclear spin-flip sidebands, with some branching ratio contrast  $\rho$  [4, 5], which causes modulations in the time-domain when measuring spin echo decays. This is known as electron spin echo envelope modulation, or ESEEM [6]. A non-zero  $\rho$  appears when the effective field on the yttrium ion depends on the state of the ytterbium ion, which comes from the fact that the expectation value  $\langle\boldsymbol{\mu}\rangle$  is state-dependent. The branching factor  $\rho$  is directly related to the angle between the two effective fields, see Refs [4, 5].

At the ZEFOZ point, the  $^{171}\text{Yb}^{3+}$  expectation value of the dipole moment is zero, i.e.  $\langle\boldsymbol{\mu}\rangle = 0$ , resulting in branching ratio contrast  $\rho = 0$  [4, 5]. Hence, to first order, there should be no ESEEM at the ZEFOZ point.

When we apply a small bias field, each state acquires a weak effective dipole moment due to the non-zero expectation value with respect to the expectation values of the perturbed eigenstates,  $\langle\tilde{\chi}|S_k|\tilde{\chi}\rangle \neq 0$ , see Eq. S.10, which activates the dipole-dipole coupling. However, as we will see in section ID,  $\langle\tilde{\chi}|S_k|\tilde{\chi}\rangle$  can be minimized by properly tuning the angle of the applied bias field, thanks to the fact that the  $\mathbf{A}$  and  $\mathbf{g}$  tensors are highly anisotropic, with their strong and weak values approximately aligned. In section ID we will derive an approximate, first-order, formula for  $\langle\tilde{\chi}|S_k|\tilde{\chi}\rangle$ , see Eq. S.23.

We anticipate this result, and note that the first-order ytterbium dipole moment can be written as  $\langle\boldsymbol{\mu}\rangle = B\xi\mathbf{e}_\mu$ , see Eq. S.26, where  $B$  is the magnitude of  $\mathbf{B}$ ,  $\xi$  a proportionality factor, and  $\mathbf{e}_\mu$  a unit vector. The linear dependence on  $B$  is expected intuitively, as the energy of each state depends quadratically on  $B$  for small fields. In addition, both  $\xi$  and  $\mathbf{e}_\mu$  depend on the state of the  $^{171}\text{Yb}^{3+}$  ion and the *orientation* of the magnetic field, but are independent of the field *magnitude*  $B$ , see Eq. S.25. If we further write  $\mathbf{r} = r\mathbf{e}_r$  and  $\mathbf{B} = B\mathbf{e}_B$ , where  $\mathbf{e}_r$  and  $\mathbf{e}_B$  are unit vectors, then we can write the effective field as

$$\mathbf{B}_Y = B \left( \mathbf{e}_B - \frac{\mu_0}{4\pi} \frac{\xi}{r^3} [\mathbf{e}_\mu - 3(\mathbf{e}_\mu \cdot \mathbf{e}_r) \cdot \mathbf{e}_r] \right) = B\mathbf{m}_\mu. \quad (\text{S.12})$$

The first-order splitting of the  $^{171}\text{Yb}^{3+}$  hyperfine state due to the interaction with an yttrium ion is then simply given by  $\Delta_Y = B|\mathbf{m}_\mu|\gamma_Y$ , where  $\gamma_Y$  is the gyromagnetic ratio of yttrium. It is quite remarkable that  $|\mathbf{m}_\mu|$  is independent of the *magnitude* of the field, due to the fact that the first-order dipole moment is linear in  $B$ , however, it is strongly dependent on the inter-ion distance  $r$ , as expected. It also depends on the state of the  $^{171}\text{Yb}^{3+}$  ion and the *orientation* of the magnetic field, through  $\xi$  and  $e_\mu$  in Eq. S.12. Numerical calculations based on the relative positions of ytterbium and yttrium ions indicate that  $|\mathbf{m}_\mu|$  rarely exceed 2 for the closest ions, and quickly converges to around 1 for ions further away ( $6 \gtrsim \text{\AA}$ ). Hence, the interaction only slightly modifies the yttrium Zeeman split (and, hence, the split of the ytterbium ion). Yet, the combined effect of a collection of ESEEM oscillations at slightly different frequencies appear to have a profound effect on the Hahn echo decay, as shown experimentally in the article.

We finally comment on two key differences when comparing the superhyperfine interaction in  $^{171}\text{Yb}^{3+}:\text{Y}_2\text{SiO}_5$  and the superhyperfine interaction with the Kramers Zeeman doublet states in  $\text{Er}^{3+}:\text{Y}_2\text{SiO}_5$ , as modeled in [4, 5]. In  $\text{Er}^{3+}:\text{Y}_2\text{SiO}_5$ , an effective screening model was invoked to explain the dependence of the dephasing time on the magnetic field strength  $B$  [5]. Such a model cannot work in  $^{171}\text{Yb}^{3+}:\text{Y}_2\text{SiO}_5$ , where the first-order dipole moment itself is also linear in the field. This is encapsulated by the fact that the  $\mathbf{m}_\mu$  vector is independent of the field magnitude  $B$  in  $^{171}\text{Yb}^{3+}:\text{Y}_2\text{SiO}_5$ . This also results in a branching ratio  $\rho$  that is independent of  $B$ , another key difference with the case studied in  $\text{Er}^{3+}:\text{Y}_2\text{SiO}_5$ . Both depend, however, on the orientation of the field, which explains why the ESEEM pattern displays a strong orientation dependence, as seen in Fig. 2(a) and (b) in the article.

#### D. Calculation of $\langle \tilde{\chi} | S_k | \tilde{\chi} \rangle$

As discussed above, the key to understanding the  $S_1$  gradient and the effective dipole moment is to calculate the expectation value  $\langle \tilde{\chi} | S_k | \tilde{\chi} \rangle$ . With the definition of  $|\tilde{\chi}\rangle$ , Eq. S.6, we find that

$$\begin{aligned} \langle \tilde{\chi} | S_k | \tilde{\chi} \rangle &= \\ & \left( \langle \chi | + \sum_{\alpha' \neq \chi} \kappa_{\alpha'} \gamma_{\alpha' \chi}^* \langle \alpha' | \right) S_k \left( | \chi \rangle + \sum_{\alpha \neq \chi} \kappa_{\alpha} \gamma_{\alpha \chi} | \alpha \rangle \right) = \\ & \langle \chi | S_k | \chi \rangle + \sum_{\alpha \neq \chi} \kappa_{\alpha} \gamma_{\alpha \chi} \langle \chi | S_k | \alpha \rangle + \sum_{\alpha' \neq \chi} \kappa_{\alpha'} \gamma_{\alpha' \chi}^* \langle \alpha' | S_k | \chi \rangle + \\ & \sum_{\alpha' \neq \chi, \alpha \neq \chi} \kappa_{\alpha'} \gamma_{\alpha' \chi}^* \kappa_{\alpha} \gamma_{\alpha \chi} \langle \alpha' | S_k | \alpha \rangle. \end{aligned} \quad (\text{S.13})$$

Note that  $\kappa_{\alpha}$  is real, given its definition. Also, the first term is  $\langle \chi | S_k | \chi \rangle = 0$ . We start by looking at the second and third terms in the equation above.

For the two sums in terms 2 and 3, we must have that  $|\alpha\rangle = |\alpha'\rangle$ , as only one other Bell state will give a non-zero overlap with  $|\chi\rangle$ , given a  $S_k$  operator (see Sec. IF). If we name this state  $|\beta\rangle$ , i.e. only  $\langle \beta | S_k | \chi \rangle \neq 0$ , then the sums in terms 2 and 3 will simply reduce to

$$\kappa_{\beta} \gamma_{\beta \chi} \langle \chi | S_k | \beta \rangle + \kappa_{\beta} \gamma_{\beta \chi}^* \langle \beta | S_k | \chi \rangle. \quad (\text{S.14})$$

Now, given the definition of  $\gamma_{\beta \chi}$  and  $\mathcal{H}_1$  we have

$$\begin{aligned} \gamma_{\beta \chi} &= \langle \beta | \mathcal{H}_1 | \chi \rangle = \\ & \mu_B B_x g_x \langle \beta | S_x | \chi \rangle + \mu_B B_y g_y \langle \beta | S_y | \chi \rangle + \mu_B B_z g_z \langle \beta | S_z | \chi \rangle = \\ & \mu_B B_k g_k \langle \beta | S_k | \chi \rangle, \end{aligned} \quad (\text{S.15})$$

where  $S_k$  is the same spin operator that appears in  $\mathcal{H}_2$ . In other words, given two Bell states  $|\chi\rangle$  and  $|\beta\rangle$ , where  $\langle \beta | S_k | \chi \rangle \neq 0$ , then only the corresponding  $S_k$  term in  $\mathcal{H}_1$  is non-zero. We can now rewrite Eq. S.14 as

$$\begin{aligned} & \kappa_{\beta} \mu_B B_k g_k (\langle \beta | S_k | \chi \rangle \langle \chi | S_k | \beta \rangle + \langle \beta | S_k | \chi \rangle^* \langle \beta | S_k | \chi \rangle) = \\ & \kappa_{\beta} \mu_B B_k g_k (\langle \beta | S_k | \chi \rangle \langle \chi | S_k | \beta \rangle + \langle \chi | S_k | \beta \rangle \langle \beta | S_k | \chi \rangle) = \\ & \kappa_{\beta} \mu_B B_k g_k 2 |\langle \beta | S_k | \chi \rangle|^2. \end{aligned} \quad (\text{S.16})$$

Here we have used the fact that the spin operators  $S_k$  are Hermitian. In general, we have that  $|\langle\beta|S_k|\chi\rangle|^2 = 1/4$ , see Sec. [IF](#), for any combination of  $S_k$ ,  $|\chi\rangle$  and  $|\beta\rangle$ , which means that terms 2 and 3 of Eq. [S.13](#) can be written as (using the definition of  $\kappa_\beta$ )

$$\frac{1}{2}\mu_B B_k g_k \frac{1}{E_\chi - E_\beta} \quad (\text{S.17})$$

where, for a given hyperfine state  $|\chi\rangle$ ,  $|\beta\rangle$  is the only hyperfine state such that  $\langle\beta|S_k|\chi\rangle \neq 0$ .

Finally, we will consider the last term in Eq. [S.13](#),

$$\sum_{\alpha' \neq \chi, \alpha \neq \chi} \kappa_{\alpha'} \gamma_{\alpha'\chi}^* \kappa_\alpha \gamma_{\alpha\chi} \langle\alpha'|S_k|\alpha\rangle. \quad (\text{S.18})$$

Indices  $\alpha$  and  $\alpha'$  run over the three other Bell states, other than the state  $|\chi\rangle$  which is of interest, so in principle it contains 9 terms. However, the last overlap function is only non-zero if  $\alpha' \neq \alpha$ , which means that there are finally 6 terms to consider. These can be grouped into three conjugate pairs of the form

$$\begin{aligned} & \kappa_{\alpha'} \gamma_{\alpha'\chi}^* \kappa_\alpha \gamma_{\alpha\chi} \langle\alpha'|S_k|\alpha\rangle + \kappa_\alpha \gamma_{\alpha\chi}^* \kappa_{\alpha'} \gamma_{\alpha'\chi} \langle\alpha|S_k|\alpha'\rangle = \\ & \kappa_{\alpha'} \kappa_\alpha (\langle\chi|\mathcal{H}_1|\alpha'\rangle \langle\alpha|\mathcal{H}_1|\chi\rangle \langle\alpha'|S_k|\alpha\rangle + \\ & \langle\alpha'|\mathcal{H}_1|\chi\rangle \langle\chi|\mathcal{H}_1|\alpha\rangle \langle\alpha|S_k|\alpha'\rangle). \end{aligned} \quad (\text{S.19})$$

We recall that, in this sum,  $|\alpha'\rangle$ ,  $|\alpha\rangle$  and  $|\chi\rangle$  must be three distinct states. As argued above, any term of the form  $\langle\chi|\mathcal{H}_1|\alpha\rangle$  can only have contribution from one of the spin operators in  $\mathcal{H}_1$ , given the states. Moreover, since  $|\alpha'\rangle$ ,  $|\alpha\rangle$  and  $|\chi\rangle$  are distinct, it follows that the corresponding spin operators must all be different, i.e. all three operators  $S_x$ ,  $S_y$  and  $S_z$  must contribute to the right and left terms in the equation above. We can then write it as

$$\begin{aligned} & \kappa_{\alpha'} \kappa_\alpha (\langle\chi|S_m|\alpha'\rangle \langle\alpha|S_n|\chi\rangle \langle\alpha'|S_k|\alpha\rangle + \\ & \langle\alpha'|S_m|\chi\rangle \langle\chi|S_n|\alpha\rangle \langle\alpha|S_k|\alpha'\rangle), \end{aligned} \quad (\text{S.20})$$

where  $m \neq n \neq k$ . Now, due to the fact that two of the spin operators have real eigenvalues ( $S_x$  and  $S_z$ ), while one has imaginary eigenvalues ( $S_y$ ), it follows that the conjugate overlap functions of two of the operators have the same sign ( $S_x$  and  $S_z$ ), while, for the third operator the conjugate overlap functions have opposite signs ( $S_y$ ), see Sec. [IF](#). For instance, if we assume  $m = x$ ,  $n = z$  and  $k = y$ , then we have

$$\kappa_{\alpha'} \kappa_\alpha \langle\chi|S_x|\alpha'\rangle \langle\alpha|S_y|\chi\rangle (\langle\alpha'|S_y|\alpha\rangle - \langle\alpha|S_y|\alpha'\rangle) = 0. \quad (\text{S.21})$$

This holds for any three distinct spin operators  $S_m$ ,  $S_n$  and  $S_k$ . Hence, the three pair-wise terms in the sum of Eq. [S.22](#) will mutually cancel each other and the total sum is zero

$$\sum_{\alpha' \neq \chi, \alpha \neq \chi} \kappa_{\alpha'} \gamma_{\alpha'\chi}^* \kappa_\alpha \gamma_{\alpha\chi} \langle\alpha'|S_k|\alpha\rangle = 0. \quad (\text{S.22})$$

It then follows that the expectation value is simply

$$\langle\tilde{\chi}|S_k|\tilde{\chi}\rangle = \frac{1}{2}\mu_B B_k g_k \frac{1}{E_\chi - E_\beta}. \quad (\text{S.23})$$

For a given direction  $k$  one must identify the state  $|\beta\rangle$  that has finite overlap with  $|\chi\rangle$  for operator  $S_k$ ,  $\langle\beta|S_k|\chi\rangle \neq 0$ , which allows to calculate the factor  $E_\chi - E_\beta$ . This equation now allows calculating the effective dipole moment vector elements for each state  $|\chi\rangle$ , see Eq. [S.10](#),

$$\langle\boldsymbol{\mu}\rangle = \frac{1}{2}\mu_B^2 (B_x g_x^2 \frac{1}{E_\chi - E_{\beta_x}}, B_y g_y^2 \frac{1}{E_\chi - E_{\beta_y}}, B_z g_z^2 \frac{1}{E_\chi - E_{\beta_z}}), \quad (\text{S.24})$$

where  $\langle \beta_k | S_k | \chi \rangle \neq 0$ . If we write the field as a vector  $\mathbf{B} = (B_x, B_y, B_z) = B(\cos(\theta) \cos(\phi), \cos(\theta) \sin(\phi), \sin(\theta))$ , where  $B$  is the magnitude,  $\phi$  the angle in the  $xy$ -plane and  $\theta$  the angle to the  $xy$ -plane, then the dipole is

$$\langle \boldsymbol{\mu} \rangle = \frac{1}{2} \mu_B^2 B (\cos(\theta) \cos(\phi) \frac{g_x^2}{E_\chi - E_{\beta_x}}, \cos(\theta) \sin(\phi) \frac{g_y^2}{E_\chi - E_{\beta_y}}, \sin(\theta) \frac{g_z^2}{E_\chi - E_{\beta_z}}). \quad (\text{S.25})$$

Hence, the first-order effective dipole moment of the yttrium ion is simply linear in the field magnitude, meaning there is no *screening* which increases with the field magnitude effect as discussed in the case of  $\text{Er}^{3+}:\text{Y}_2\text{SiO}_5$  in Ref. [7]. The dipole moment can thus be written as

$$\langle \boldsymbol{\mu} \rangle = B \xi \mathbf{e}_\mu \quad (\text{S.26})$$

where  $\mathbf{e}_\mu$  is a unit vector and  $\xi$  a scaling constant. It should be emphasized that both  $\mathbf{e}_\mu$  and  $\xi$  depend on the *orientation* of the magnetic field, but are independent of the *magnitude* of the field. These factors only needs to be calculated once for each ion, given the field orientation.

As for the energy gradient, according to Eq. S.9, state  $|\chi\rangle$  will have the following gradient along direction  $k$ ,

$$\frac{dE_\chi}{dB_k} = \frac{1}{2} \mu_B^2 B_k g_k^2 \frac{1}{E_\chi - E_\beta}. \quad (\text{S.27})$$

To derive a formula for  $S_1$ , one needs to consider the two states involved in the relevant transition  $T$ . For each state  $|\chi\rangle$ , the gradient is calculated for each direction  $k = x, y, z$  using the equation above.

### E. $S_1$ gradient of the 2.497 GHz transition

Following the method of calculation outlined in the previous section, one can derive the  $S_1$  gradient of the 2.497 GHz transition connecting the  $|\psi^+\rangle$  and  $|\phi^-\rangle$  states:

$$S_1 = 2\mu_b^2 \sqrt{\frac{B_x^2 g_x^4 A_z^2}{(A_y^2 - A_z^2)^2} + \frac{B_y^2 g_y^4}{(A_x - A_z)^2} + \frac{B_z^2 g_z^4 A_x^2}{(A_x^2 - A_y^2)^2}}. \quad (\text{S.28})$$

The gradient is highly suppressed when aligning the field in the  $x$  direction, due to the low numerator and high denominator, as  $A_x \ll A_y \ll A_z$  and  $g_x \ll g_y \ll g_z$ . In general, as pointed out in [8], the gradient is low in the entire  $xy$ -plane.

In optics experiments in  $\text{Y}_2\text{SiO}_5$ , it is convenient to work in the  $D_1$ - $D_2$  plane, where  $D_1$  and  $D_2$  are two polarization extinction axes [9], as in this plane the two magnetic sub sites (related by a  $C_2$  rotation around  $b$ ) become equivalent. The minimum gradient in the  $D_1$ - $D_2$  plane is therefore expected where the  $xy$ -plane intersects the  $D_1$ - $D_2$  plane. Given the  $\mathbf{g}$  tensor of the ground state of site II [2], it follows that the intersection is at about 59 deg from the  $D_1$  axis. In Fig. S2, a full numerical computation of the  $S_1$  gradient is compared to the analytical result, Eq. S.28, showing a good agreement. The numerical calculation is minimum for the exact angle of 55.9 deg to the  $D_1$  axis.

Finally, we compare the  $S_1$  gradient for all spin transitions in the  $D_1$ - $D_2$  plane, see Fig. S3. As can be seen, all transitions have their minima around the  $xy$ -plane intersection with the  $D_1$ - $D_2$  plane. The 2.497 GHz and 2.370 GHz transition gradients are indistinguishable on this scale, as are the gradients for the 1.842 GHz and 3.025 GHz transitions. The 529 MHz and 655 MHz transitions are clearly distinguishable in the high gradient region. Notably, the 2.497 GHz and 2.370 GHz gradients vary much less in general, which we experienced also in the lab, as the 2.497 GHz transition was less sensitive to different spurious bias fields in the lab, as compared to our past experience when working with the 655 MHz transition [8, 10].

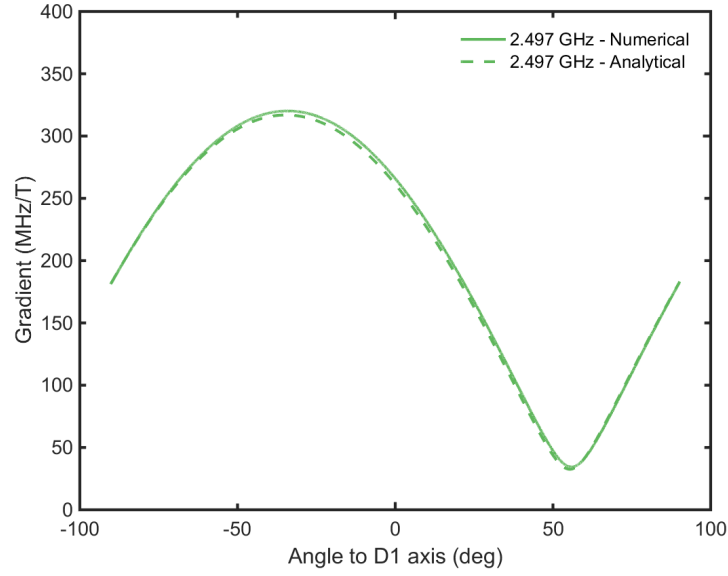

FIG. S2. The  $S_1$  gradient of the 2.497 GHz transition as a function of the angle in the  $D_1$ - $D_2$  plane, calculated for a fixed field magnitude of 1 milli-Tesla. The solid line show the numerical calculation of the gradient, with the full  $\mathbf{g}$  [2] and  $\mathbf{A}$  [1] tensors. The dashed line shows the gradient computed with the approximate analytical formula, Eq. S.28, where the  $\mathbf{g}$  and  $\mathbf{A}$  tensors are assumed to be aligned.

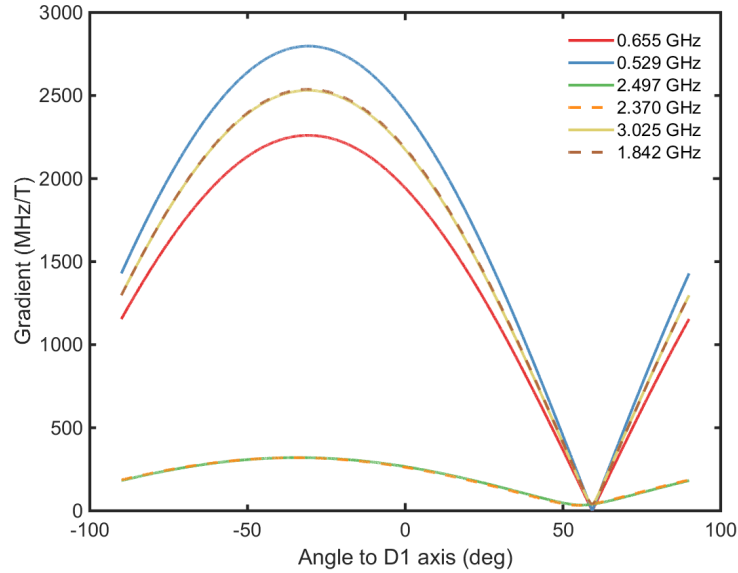

FIG. S3. Numerical calculations of the  $S_1$  gradient for all the ground-state spin transitions, as a function of the angle in the  $D_1$ - $D_2$  plane (field magnitude 1 milli-Tesla).

### F. Some spin operator properties

Here, we give useful tables of how the  $S_x$ ,  $S_y$  and  $S_z$  operators act on the four Bell states. We recall that these operators are of the form  $S_k \otimes 1$ , hence the nuclear spin is unaffected.

$$\begin{aligned}
S_z |\phi^+\rangle &= \frac{1}{2} |\phi^-\rangle, \\
S_z |\phi^-\rangle &= \frac{1}{2} |\phi^+\rangle, \\
S_z |\psi^+\rangle &= \frac{1}{2} |\psi^-\rangle, \\
S_z |\psi^-\rangle &= \frac{1}{2} |\psi^+\rangle,
\end{aligned} \tag{S.29}$$

$$\begin{aligned}
S_x |\phi^+\rangle &= \frac{1}{2} |\psi^+\rangle, \\
S_x |\phi^-\rangle &= -\frac{1}{2} |\psi^-\rangle, \\
S_x |\psi^+\rangle &= \frac{1}{2} |\phi^+\rangle, \\
S_x |\psi^-\rangle &= -\frac{1}{2} |\phi^-\rangle,
\end{aligned} \tag{S.30}$$

$$\begin{aligned}
S_y |\phi^+\rangle &= \frac{1}{2i} |\psi^-\rangle, \\
S_y |\phi^-\rangle &= -\frac{1}{2i} |\psi^+\rangle, \\
S_y |\psi^+\rangle &= \frac{1}{2i} |\phi^-\rangle, \\
S_y |\psi^-\rangle &= -\frac{1}{2i} |\phi^+\rangle.
\end{aligned} \tag{S.31}$$

From this, it follows that any two distinct Bell states  $|\chi_1\rangle$  and  $|\chi_2\rangle$  obey

$$\begin{aligned}
\langle \chi_1 | S_x | \chi_2 \rangle &= \langle \chi_2 | S_x | \chi_1 \rangle, \\
\langle \chi_1 | S_z | \chi_2 \rangle &= \langle \chi_2 | S_z | \chi_1 \rangle, \\
\langle \chi_1 | S_y | \chi_2 \rangle &= -\langle \chi_2 | S_y | \chi_1 \rangle,
\end{aligned} \tag{S.32}$$

## II. EFFECTIVE SPIN DEPHASING TIME $T_2$ AS A FUNCTION OF FIELD STRENGTH ALONG THE $D_1$ AXIS

To extract an effective spin dephasing time  $T_2$  from the decay curves shown in Figs 2(d) and 2(e) of the article, the curves were fitted up to the first collapse of the signal, before the appearance of the first ESEEM peak. This first collapse of each curve displays a clear non-exponential time-dependence at higher fields, which can be well fitted by a stretched exponential (or Mims law). The resulting  $T_2$  are plotted in Fig. S4. The data can be fitted by the same model used for the  $b$ -axis scan,  $T_2(B) = 1/(1/T_2(0) + \pi\kappa|B - B_0|)$ , with the difference that here we fix  $B_0 = 0$  as the curve presents no maximum. We find  $T_2(0) = 12.5 \pm 0.8$  ms and  $\kappa = (1.03 \pm 0.05)\text{MHz/T}$ .

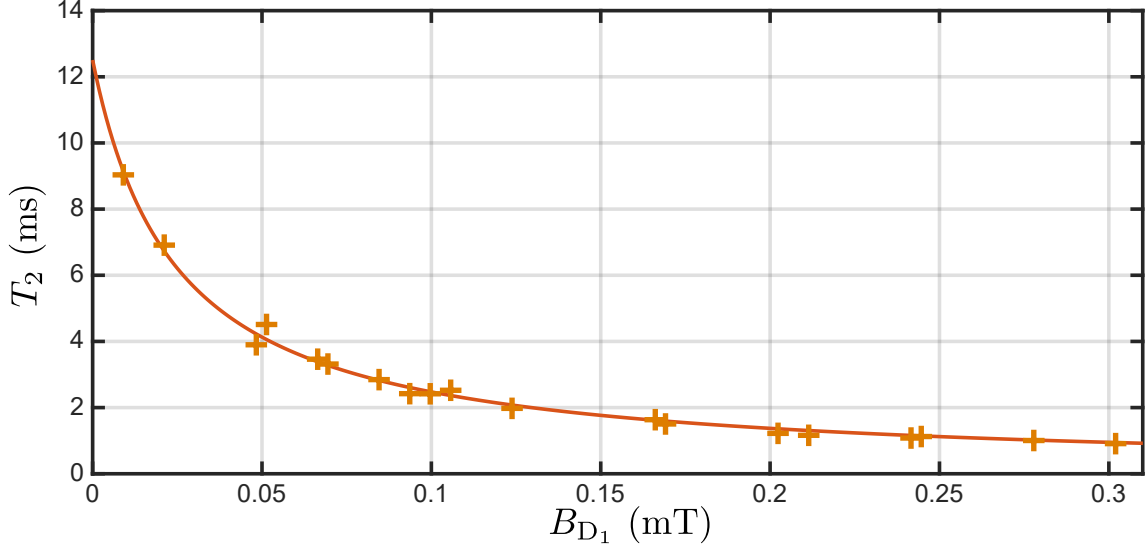

FIG. S4. Effective spin dephasing times measured along the  $D_1$  axis, see the data presented in Figs 2(d) and 2(e) of the article. The  $T_2$  is estimated from only fitting the first points of the decay curve, excluding the first ESEEM revival. The solid line shows a simple empirical model, see the text.

### III. OPTICAL COHERENCE TIME MEASUREMENTS

In addition to the spin echo measurements presented in the article, the optical coherence time was also measured on the  $|4_g\rangle\text{--}|1_e\rangle$  transition. To this end, we used a standard two pulse photon echo (PE) scheme, where the  $\pi/2$  and  $\pi$  pulses were separated by a time  $\tau_{12}$ . The PE was measured in the same  $\text{Y}_2\text{SiO}_5$  crystal as used in the main article, doped with 2 ppm of  $^{171}\text{Yb}^{3+}$ . In addition, we here show the PE data obtained in the crystal doped with 5 ppm of  $^{171}\text{Yb}^{3+}$ . The optical coherence time in the 5 ppm crystal was mentioned in Ref. [10], but without showing the PE decay curve.

In Fig.S5, we show the decay of the normalized echo intensity as a function of  $\tau_{12}$  for both doping concentrations. Both decay curves could be fitted to an exponential function  $I(\tau_{12}) = I_0 \exp(4\tau_{12}/T_2)$ , where  $T_2$  is the optical coherence time. For the 5 ppm sample we obtained  $T_2 = 610 \mu\text{s} \pm 50 \mu\text{s}$ , and for the 2 ppm sample we obtained  $T_2 = 1050 \mu\text{s} \pm 130 \mu\text{s}$ . For both crystals, we applied a small magnetic field to compensate for spurious lab bias magnetic fields, including the earth magnetic field, in order to reach the ZEFOZ point. The magnetic field was optimized by increasing the echo intensity at long delays, as in the case of the spin echo signal, see discussion in the main article.

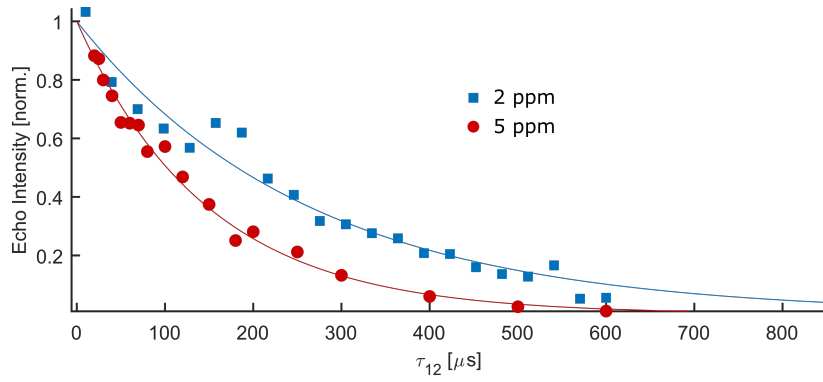

FIG. S5. Photon echo decay curves measured in two  $\text{Y}_2\text{SiO}_5$  crystals with 5 ppm (red circles) and 2 ppm (blue squares) of  $^{171}\text{Yb}^{3+}$  concentration. The fitted optical coherence times are  $T_2 = 610 \mu\text{s} \pm 50 \mu\text{s}$  and  $T_2 = 1050 \mu\text{s} \pm 130 \mu\text{s}$ , for the 5 and 2 ppm samples, respectively.

#### IV. OPTICAL BRANCHING RATIOS AND $\Lambda$ -SYSTEMS

The optical branching ratio table, involving all possible optical transitions between the hyperfine states of the  $^2F_{7/2}(0) \longleftrightarrow ^2F_{5/2}(0)$  optical transition, is a key parameter for quantum memory applications. The table for site II with the optical polarization along the  $D_2$  axis was published in the Supplementary Materials of Ref. [10]. Here, we complement those data with the corresponding tables for the optical polarization along the  $D_1$  and  $b$  axes, see Table IV. The measurement method is the same as the one used in Ref. [10]. The hyperfine states are indicated using the notation in Fig. 1 of the main article.

The branching table depends on the polarization of the optical excitation, which allows one to tailor efficient  $\Lambda$ -systems for quantum memory experiments. A  $\Lambda$ -system couples two ground-level hyperfine states to a common excited hyperfine state, ideally through two transitions with high transition strengths. Table IV shows that efficient  $\Lambda$ -systems can be formed using different polarizations for the two transitions, specifically along the  $D_2$  and  $b$  axes. An efficient  $\Lambda$ -system involving the 2.497 GHz transition studied in this work can be formed using  $|2_g\rangle \leftrightarrow |1_e\rangle$  and  $|1_e\rangle \leftrightarrow |4_g\rangle$ , with relative oscillator strengths 0.21 (along  $b$ ) and 0.72 (along  $D_2$ ), respectively. A particularly interesting  $\Lambda$ -system involves the highest spin transition at 3.0 GHz, using  $|1_g\rangle \leftrightarrow |4_e\rangle$  and  $|4_e\rangle \leftrightarrow |4_g\rangle$ , with relative oscillator strengths 0.71 (along  $D_2$ ) and 0.61 (along  $b$ ), respectively. An alternative is to couple the ground states through the excited state  $|1_e\rangle$ . Similarly one can form two efficient  $\Lambda$ -systems involving the 1.842 GHz spin transition (involving  $|2_g\rangle$  and  $|3_g\rangle$ ), through either the excited  $|2_e\rangle$  or  $|3_e\rangle$ .

In terms of relative transition strengths, all the possible  $\Lambda$ -systems mentioned above are better than any other possibility involving two transitions with the same polarization. The number of possible efficient  $\Lambda$ -systems is highly interesting, as it allows optimizing the quantum memory scheme in terms of other key parameters, such as optical and spin coherence times, and optical memory bandwidth (see discussion in Ref. [10]).

TABLE I. Measured relative optical oscillator strengths for  $^{171}\text{Yb}^{3+}:\text{Y}_2\text{SiO}_5$  optical  $^2F_{7/2}(0) \longleftrightarrow ^2F_{5/2}(0)$  transition for crystallographic site II measured for light polarized along  $D_1$ ,  $D_2$  and  $b$  axes.

| $\vec{E} \parallel D_1$ |               |               |               |               | $\vec{E} \parallel D_2$ |               |               |               |               | $\vec{E} \parallel b$ |               |               |               |               |
|-------------------------|---------------|---------------|---------------|---------------|-------------------------|---------------|---------------|---------------|---------------|-----------------------|---------------|---------------|---------------|---------------|
| $ 1_g\rangle$           | $ 1_e\rangle$ | $ 2_e\rangle$ | $ 3_e\rangle$ | $ 4_e\rangle$ | $ 1_g\rangle$           | $ 1_e\rangle$ | $ 2_e\rangle$ | $ 3_e\rangle$ | $ 4_e\rangle$ | $ 1_g\rangle$         | $ 1_e\rangle$ | $ 2_e\rangle$ | $ 3_e\rangle$ | $ 4_e\rangle$ |
| 0.15                    | 0.15          | 0.05          | 0.64          |               | 0.15                    | 0.06          | 0.08          | 0.71          |               | 0.54                  | 0.19          | 0.03          | 0.24          |               |
| $ 2_g\rangle$           | 0.16          | 0.19          | 0.63          | 0.02          | $ 2_g\rangle$           | 0.06          | 0.19          | 0.71          | 0.04          | $ 2_g\rangle$         | 0.21          | 0.57          | 0.21          | 0.01          |
| $ 3_g\rangle$           | 0.01          | 0.61          | 0.22          | 0.16          | $ 3_g\rangle$           | 0.07          | 0.71          | 0.16          | 0.06          | $ 3_g\rangle$         | 0.01          | 0.18          | 0.66          | 0.15          |
| $ 4_g\rangle$           | 0.69          | 0.05          | 0.09          | 0.189         | $ 4_g\rangle$           | 0.72          | 0.04          | 0.05          | 0.19          | $ 4_g\rangle$         | 0.23          | 0.06          | 0.10          | 0.61          |

- [1] A. Tiranov, A. Ortu, S. Welinski, A. Ferrier, P. Goldner, N. Gisin, and M. Afzelius, Spectroscopic study of hyperfine properties in  $^{171}\text{Yb}^{3+}:\text{Y}_2\text{SiO}_5$ , *Phys. Rev. B* **98**, 195110 (2018).
- [2] S. Welinski, A. Ferrier, M. Afzelius, and P. Goldner, High-resolution optical spectroscopy and magnetic properties of  $\text{Yb}^{3+}$  in  $\text{Y}_2\text{SiO}_5$ , *Phys. Rev. B* **94**, 155116 (2016).
- [3] J. J. Longdell, A. L. Alexander, and M. J. Sellars, Characterization of the hyperfine interaction in europium-doped yttrium orthosilicate and europium chloride hexahydrate, *Phys. Rev. B* **74**, 195101 (2006).
- [4] B. Car, L. Veissier, A. Louchet-Chauvet, J.-L. Le Gouët, and T. Chanelière, Selective optical addressing of nuclear spins through superhyperfine interaction in rare-earth doped solids, *Physical review letters* **120**, 197401 (2018).
- [5] B. Car, J.-L. Le Gouët, and T. Chanelière, Superhyperfine induced photon-echo collapse of erbium in  $\text{Y}_2\text{SiO}_5$ , *Physical Review B* **102**, 115119 (2020).
- [6] L. Rowan, E. Hahn, and W. Mims, Electron-spin-echo envelope modulation, *Physical Review* **137**, A61 (1965).
- [7] B. Car, J.-L. Le Gouët, and T. Chanelière, Superhyperfine induced photon-echo collapse of erbium in  $\text{Y}_2\text{SiO}_5$ , *Physical Review B* **102**, 115119 (2020).
- [8] A. Ortu, A. Tiranov, S. Welinski, F. Froewis, N. Gisin, A. Ferrier, P. Goldner, N. Gisin, and M. Afzelius, Simultaneous coherence enhancement of optical and microwave transitions in solid-state electronic spins, *Nature Materials* **17**, 671 (2018).
- [9] C. Li, C. Wyon, and R. Moncorge, *IEEE Journal of Quantum Electronics* **28**, 1209 (1992).
- [10] M. Businger, A. Tiranov, K. Kaczmarek, S. Welinski, Z. Zhang, A. Ferrier, P. Goldner, and M. Afzelius, Optical spin-wave storage in a solid-state hybridized electron-nuclear spin ensemble, *Physical Review Letters* **124**, 053606 (2020).
